# Supplementary material for: Recorp: Receiver-Oriented Policies for Industrial Wireless Networks
Source: arXiv:2008.09214 source file (2021-06-06)
Supplement: Supplementary file 1 [file appendix.tex]

% !TEX root = main.tex
% \section*{Appendix}

% \subsection{Correctness Proof}
% \label{sec:proof:correctness}

\input{th_wellformed.tex}
\input{proof_wellformed.tex}
